# Supplementary material for: Many Ways to Be Lonely: Fine-Grained Characterization of Loneliness and Its Potential Changes in COVID-19
Source: arXiv:2201.07423 source file (2022-04-16)
Supplement: Supplementary file 1 [file supp.tex]

\section*{\hfil Supplementary Materials\hfil} %for Submission \\\textit{\papertitle}}

\setcounter{table}{0}
\begin{table*}[ht!]

    \centering
\begin{tabular}{@{}cccccc@{}}
\toprule
                    & Acc. $\uparrow$              & Clark $\downarrow$           & Canberra $\downarrow$                 & Cosine $\uparrow$            & Intersection $\uparrow$      \\ \midrule
\multicolumn{6}{c}{Duration}                                                                                                                                                            \\ \midrule
LSTM Baseline       & 0.4059 $\pm$ 0.0018          & \textbf{1.4491 $\pm$ 0.0009} & 2.5259 $\pm$ 0.0053                   & 0.6860 $\pm$ 0.0017          & 0.5192 $\pm$ 0.0013          \\
BERT + MLP          & \textbf{0.5992 $\pm$ 0.0114} & 1.4682 $\pm$ 0.0060          & 2.5670 $\pm$ 0.0065                   & \textbf{0.7389 $\pm$ 0.0058} & \textbf{0.5713 $\pm$ 0.0113} \\
HDLN ($\beta = 0$)  & 0.4539 $\pm$ 0.0073          & 1.4622 $\pm$ 0.0057          & 2.5515 $\pm$ 0.0112                   & 0.6847 $\pm$ 0.0033          & 0.5293 $\pm$ 0.0017          \\
HDLN ($\beta = .5$) & 0.4578 $\pm$ 0.0073          & 1.4565 $\pm$ 0.0055          & 2.5364  $\pm$ 0.1229                  & 0.6894 $\pm$ 0.0024          & 0.5297 $\pm$ 0.0026          \\
HDLN ($\beta = 1$)  & 0.4552 $\pm$ 0.0095          & 1.4525 $\pm$ 0.0049          & \textbf{2.5247 $\pm$ 0.1208}          & 0.6919 $\pm$ 0.0013          & 0.5295 $\pm$ 0.0039          \\ \midrule
\multicolumn{6}{c}{Context}                                                                                                                                                             \\ \midrule
LSTM Baseline       & 0.7198 $\pm$ 0.0000          & 1.9656 $\pm$ 0.0005          & 4.1024 $\pm$ 0.0003                   & 0.7747 $\pm$ 0.0007          & 0.5643 $\pm$ 0.0038          \\
BERT + MLP          & 0.8573 $\pm$ 0.0102          & \textbf{1.9507 $\pm$ 0.0028} & \textit{\textbf{3.9649 $\pm$ 0.0083}} & \textbf{0.9065 $\pm$ 0.0051} & \textbf{0.7864 $\pm$ 0.0028} \\
HDLN ($\beta = 0$)  & 0.8560 $\pm$ 0.0220          & 1.9590 $\pm$ 0.0018          & 3.9986 $\pm$ 0.0066                   & 0.8920 $\pm$ 0.0093          & 0.7720 $\pm$ 0.0090          \\
HDLN ($\beta = .5$) & 0.8573 $\pm$ 0.0174          & 1.9577 $\pm$ 0.0013          & 3.9979 $\pm$ 0.0047                   & 0.8926 $\pm$ 0.0072          & 0.7654 $\pm$ 0.0096          \\
HDLN ($\beta = 1$)  & \textbf{0.8586 $\pm$ 0.0163} & 1.9575 $\pm$ 0.0017          & 4.0010 $\pm$ 0.0055                   & 0.8919 $\pm$ 0.0056          & 0.7577 $\pm$ 0.0109          \\ \midrule
\multicolumn{6}{c}{Interpersonal}                                                                                                                                                       \\ \midrule
LSTM Baseline       & 0.5758 $\pm$ 0.0000          & 1.9369 $\pm$ 0.0010          & 4.1178 $\pm$ 0.0048                   & 0.5742 $\pm$ 0.0051          & 0.3370 $\pm$ 0.0030          \\
BERT + MLP          & \textbf{0.7976 $\pm$ 0.0031} & 1.9077 $\pm$ 0.0009          & \textbf{3.8672 $\pm$ 0.0034}          & \textbf{0.8737 $\pm$ 0.0017} & \textbf{0.7229 $\pm$ 0.0006} \\
HDLN ($\beta = 0$)  & 0.7795 $\pm$ 0.0191          & 1.9123 $\pm$ 0.0015          & 3.8911 $\pm$ 0.0102                   & 0.8542 $\pm$ 0.0088          & 0.6943 $\pm$ 0.0148          \\
HDLN ($\beta = .5$) & 0.7665 $\pm$ 0.0145          & 1.9068 $\pm$ 0.0027          & 3.8776 $\pm$ 0.0126                   & 0.8563 $\pm$ 0.0099          & 0.6835 $\pm$ 0.0147          \\
HDLN ($\beta = 1$)  & 0.7639 $\pm$ 0.0120          & \textbf{1.9054 $\pm$ 0.0031} & 3.8774 $\pm$ 0.0131                   & 0.8510 $\pm$ 0.0102          & 0.6691 $\pm$ 0.0144          \\ \midrule
\multicolumn{6}{c}{Interaction}                                                                                                                                                         \\ \midrule
LSTM Baseline       & 0.6459 $\pm$ 0.0000          & 2.0000 $\pm$ 0.0005          & 4.2184 $\pm$ 0.0006                   & 0.7282 $\pm$ 0.0005          & 0.5384 $\pm$ 0.0023          \\
BERT + MLP          & \textbf{0.8352 $\pm$ 0.0120} & \textbf{1.9643 $\pm$ 0.0029} & \textbf{4.0096 $\pm$ 0.0112}          & \textbf{0.8852 $\pm$ 0.0084} & \textbf{0.7612 $\pm$ 0.0044} \\
HDLN ($\beta = 0$)  & 0.7237 $\pm$ 0.0138          & 1.9817 $\pm$ 0.0014          & 4.1003 $\pm$ 0.0063                   & 0.8154 $\pm$ 0.0072          & 0.6721 $\pm$ 0.0063          \\
HDLN ($\beta = .5$) & 0.7185 $\pm$ 0.0097          & 1.9826 $\pm$ 0.0011          & 4.1073 $\pm$ 0.0050                   & 0.8090 $\pm$ 0.0075          & 0.6627 $\pm$ 0.0064          \\
HDLN ($\beta = 1$)  & 0.7133 $\pm$ 0.0120          & 1.9849 $\pm$ 0.0010          & 4.1170 $\pm$ 0.0039                   & 0.7990 $\pm$ 0.0084          & 0.6529 $\pm$ 0.0064          \\ \bottomrule
\end{tabular}
    \vspace{-.5em}
    \caption{Evaluation results for fine-grained loneliness learning tasks. $\uparrow$ ($\downarrow$) indicates higher (lower) values are better. Metrics definitions can be found in Table~\ref{tab:metrics_calc} in the main submission. %\todo{update accordingly} \yunfan{DONE}
    }
  \vspace{-2em}
  \end{table*}

\setcounter{figure}{0}

\begin{figure}[ht!]

  \centering
  \includegraphics[width=0.8\textwidth, center]{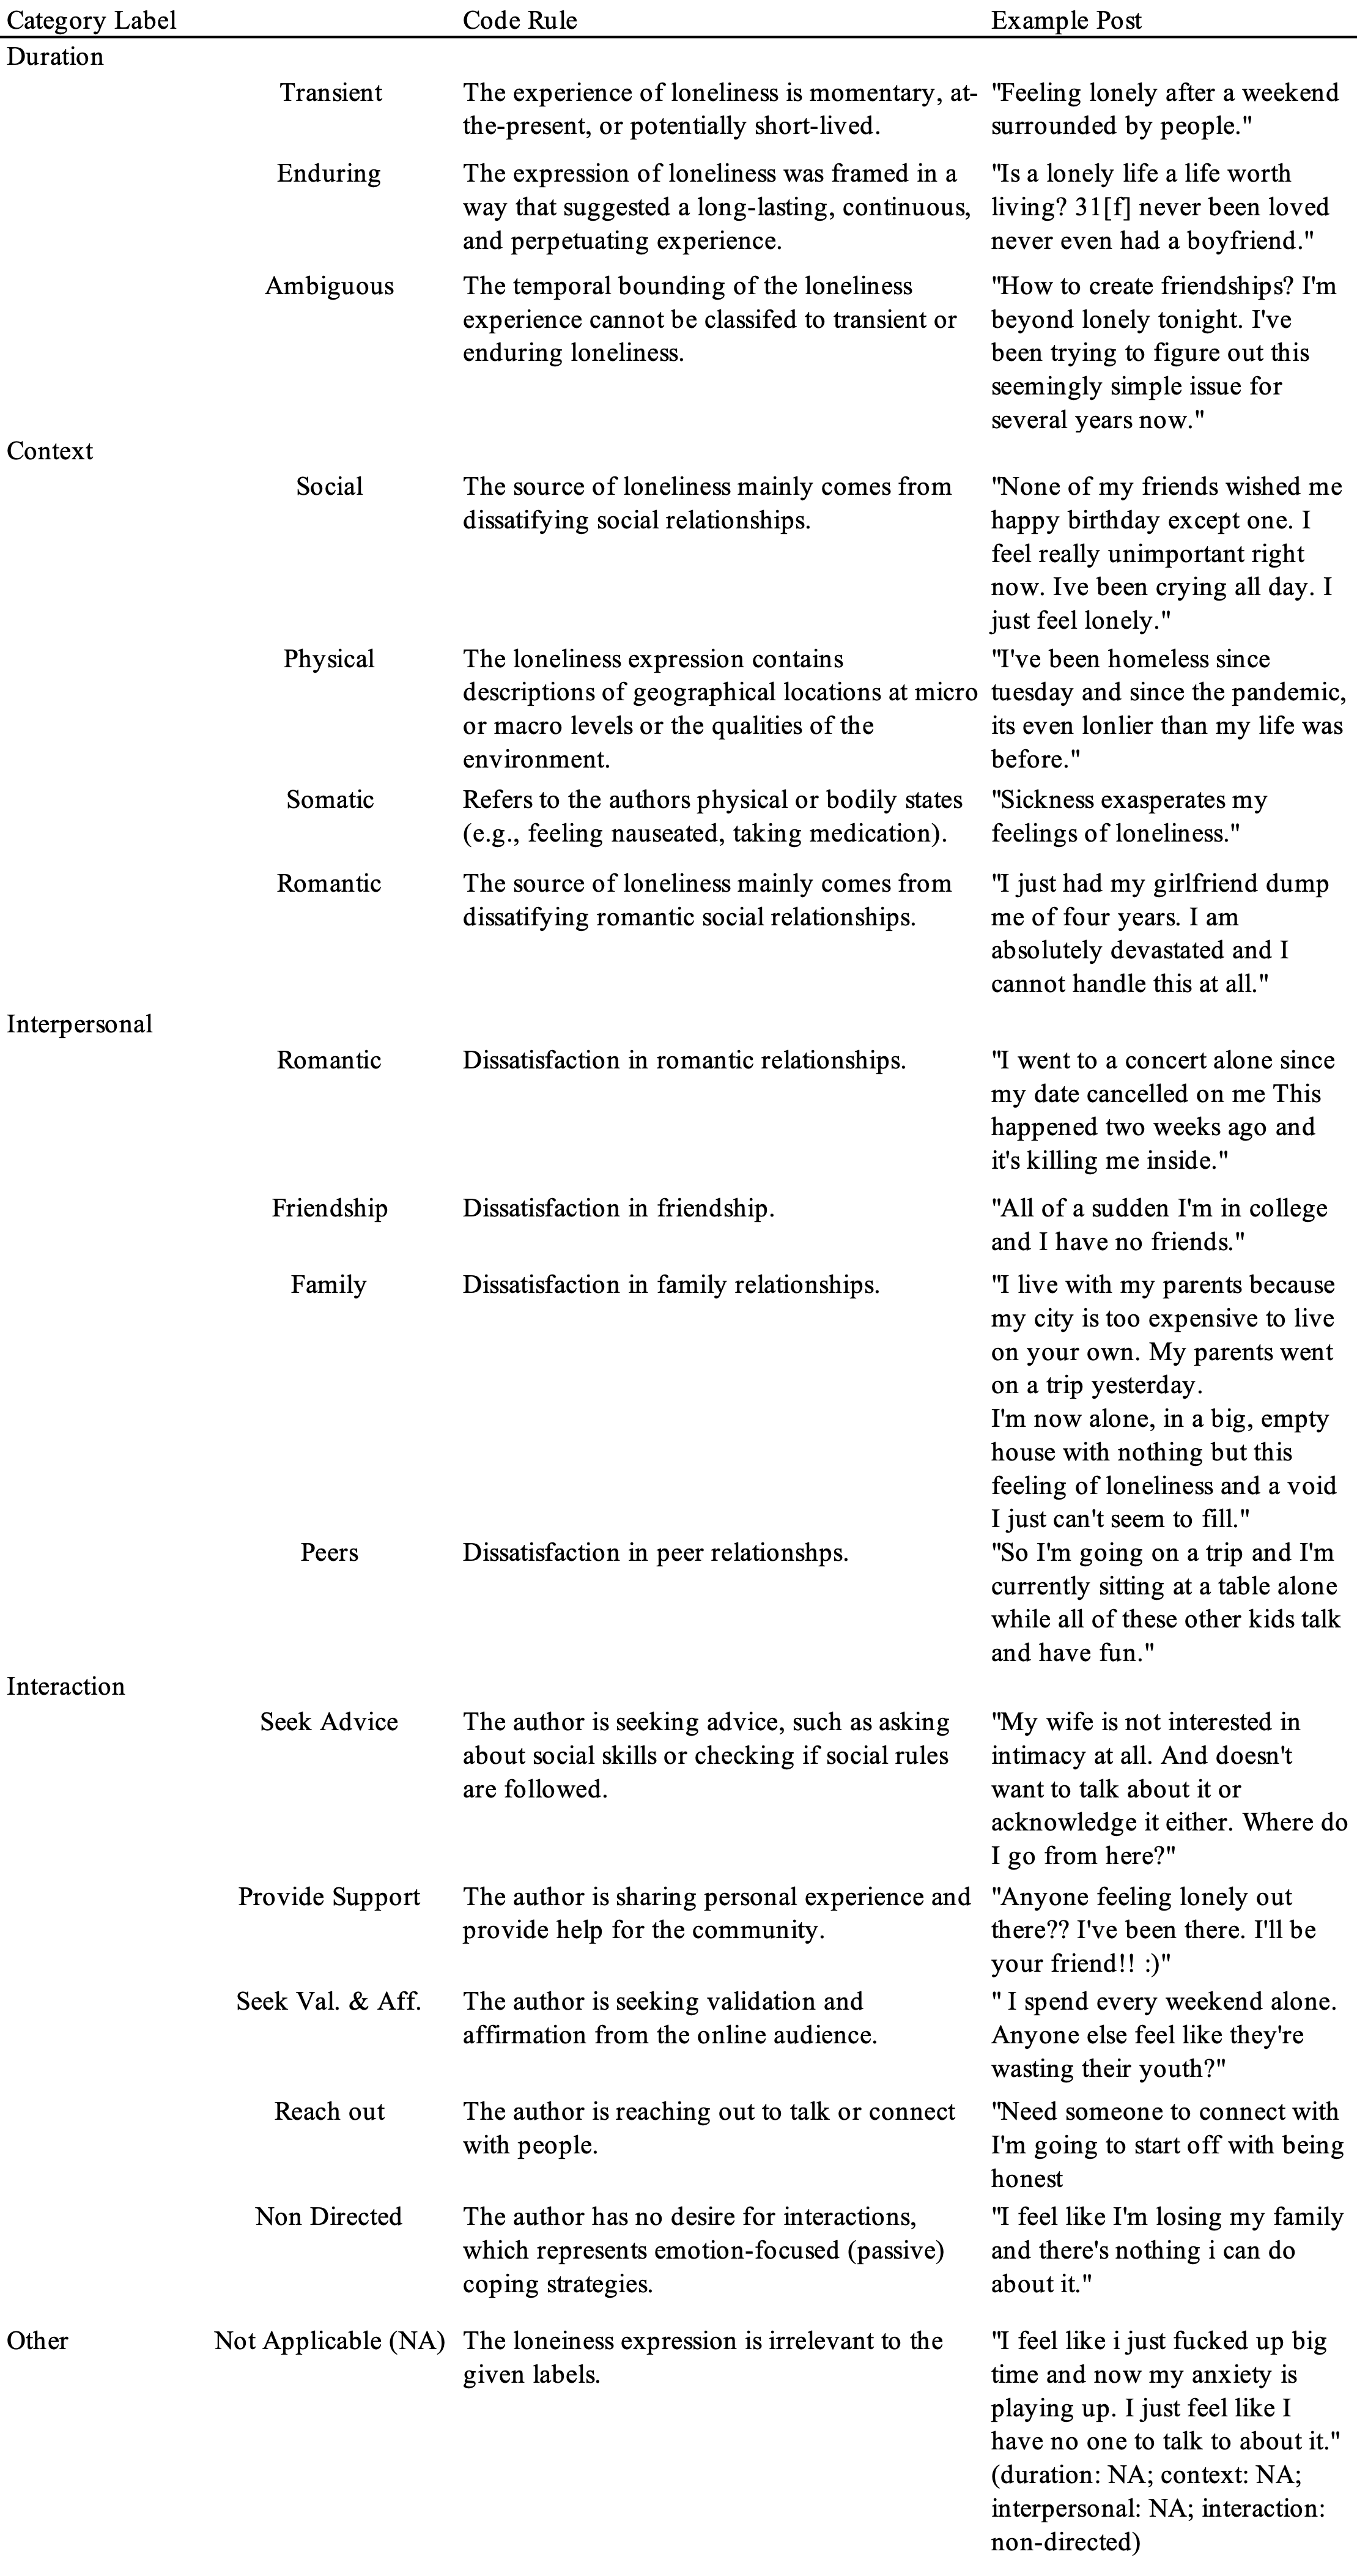}
  \caption{Codebook for annotations. Example posts were drawn from FIG-Loneliness.} 
  \label{fig:codebook}
\end{figure}
